# Supplementary material for: Origin of pressure-induced anomalies in the nodal-line ferrimagnet Mn$_3$Si$_2$Te$_6$
Source: arXiv:2509.18238 source file (2026-04-01)
Supplement: Supplementary file 1 [file supplement.pdf]

# Origin of pressure-induced anomalies in the nodal-line ferrimagnet $\text{Mn}_3\text{Si}_2\text{Te}_6$ – Supplemental Material –

Varun Venkatasubramanian,<sup>1</sup> Makoto Shimizu,<sup>2</sup> Daniel Guterding,<sup>3</sup> and Harald O. Jeschke<sup>1</sup>

<sup>1</sup>Research Institute for Interdisciplinary Science, Okayama University, Okayama 700-8530, Japan

<sup>2</sup>Department of Physics, Graduate School of Science, Kyoto University, Kyoto 606-8502, Japan

<sup>3</sup>Technische Hochschule Brandenburg, Magdeburger Straße 50, 14770 Brandenburg an der Havel, Germany

## I. ADDITIONAL DFT RESULTS

In Figs. S1 and S2, we present the structural information that is the basis for all further calculations. Lattice parameters as function of pressure are taken from experiment and interpolated. For the trigonal  $P\bar{3}1c$  phase, internal coordinates are optimized with a generic DFT+U functional in the ferromagnetic state. Relaxation in ferrimagnetic state yields very similar results.

For the monoclinic structure, we find that structure relaxation takes the internal coordinates too far away from the experimentally determined ones. Therefore, we only vary the lattice parameters as shown in Fig. S2 and keep the internal coordinates fixed at the values of the  $P = 22.3$  GPa experimental structure. The corresponding bond lengths are shown in Fig. S3.

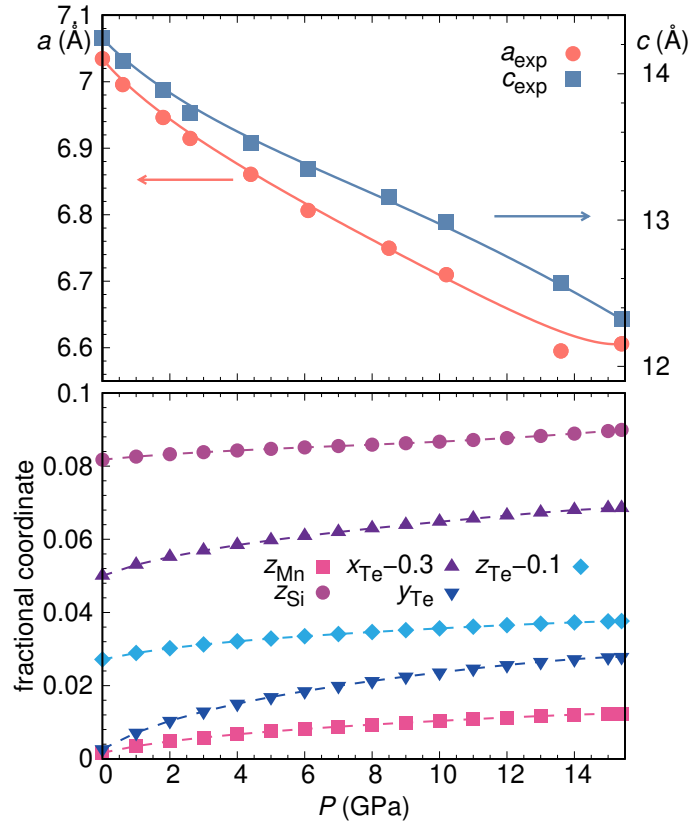

FIG. S1. Structure parameters of  $\text{Mn}_3\text{Si}_2\text{Te}_6$  as a function of pressure for the  $P\bar{3}1c$  space group. (a) Interpolated lattice parameters; symbols are experimental points taken from Ref. 1. Lines are smooth interpolations that were used for this study. (b) Fractional coordinates of  $\text{Mn}_3\text{Si}_2\text{Te}_6$  determined by relaxation of the structures with a DFT+U functional at  $U = 5$  eV in a ferromagnetic state. Dashed lines are guides to the eye.

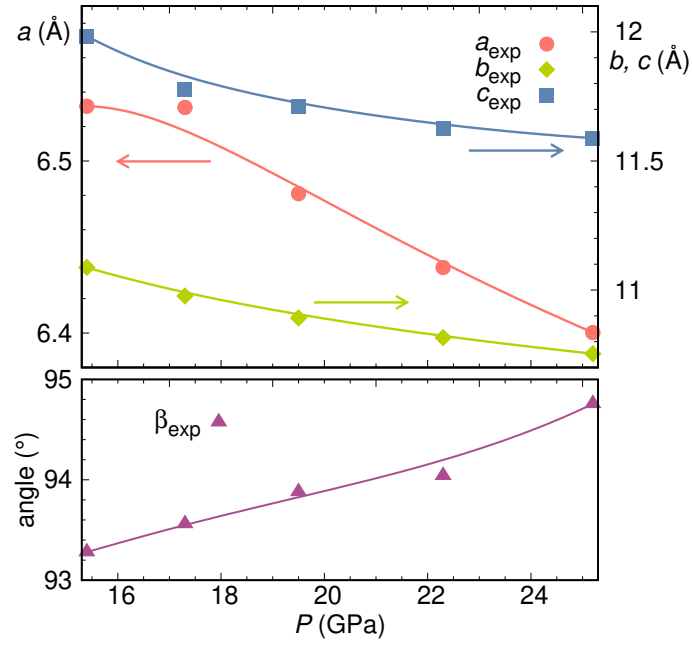

FIG. S2. Structure parameters of  $\text{Mn}_3\text{Si}_2\text{Te}_6$  as a function of pressure for the  $C2/c$  space group. (a) Interpolated lattice parameters and (b) monoclinic  $\beta$  angle; symbols are experimental points taken from Ref. 1. Lines are smooth interpolations that were used for this study.

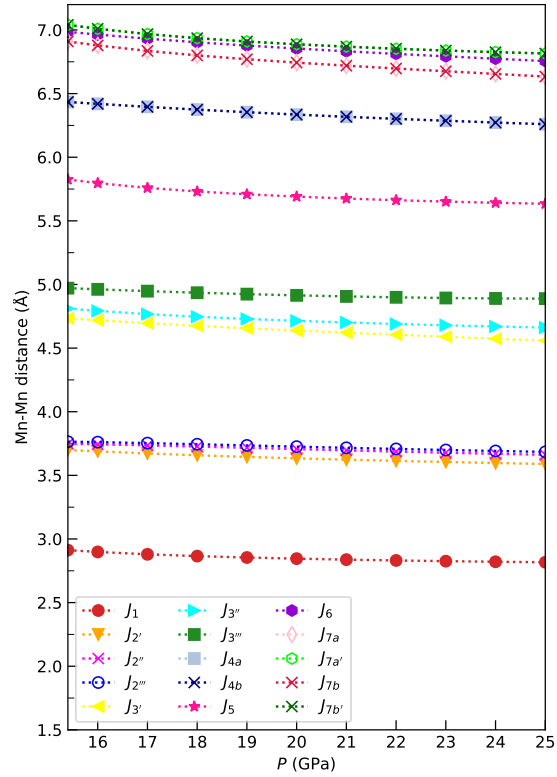

FIG. S3. Evolution of the nearest neighbour Mn-Mn distances as a function of pressure for the monoclinic structures of  $\text{Mn}_3\text{Si}_2\text{Te}_6$ .

## II. ADDITIONAL MONTE CARLO RESULTS

We present the calculated specific heat for trigonal and monoclinic structures of  $\text{Mn}_3\text{Si}_2\text{Te}_6$  in Figures S4 and S5. We use the position of the maxima to determine the ferrimagnetic ordering temperatures plotted in Fig. 4 of the main text.

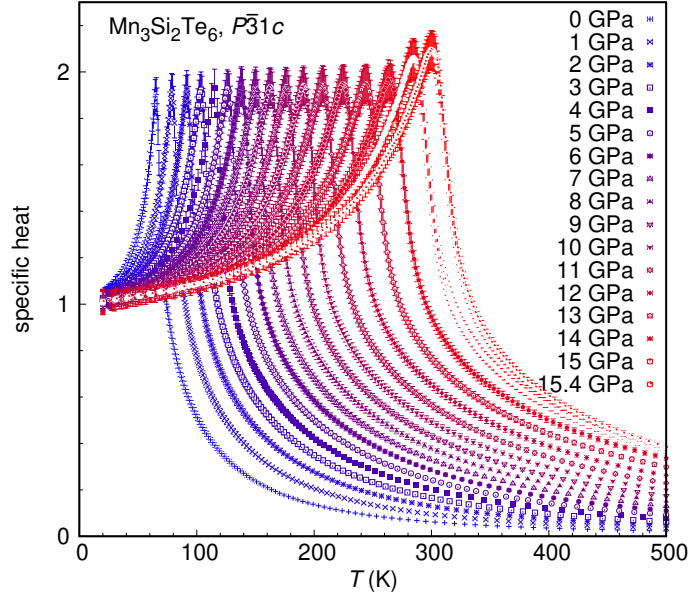

FIG. S4. Specific heat for the trigonal  $P\bar{3}1c$  structure of  $\text{Mn}_3\text{Si}_2\text{Te}_6$ . Pressures range from  $P = 0$  to  $P = 15.4$  GPa.

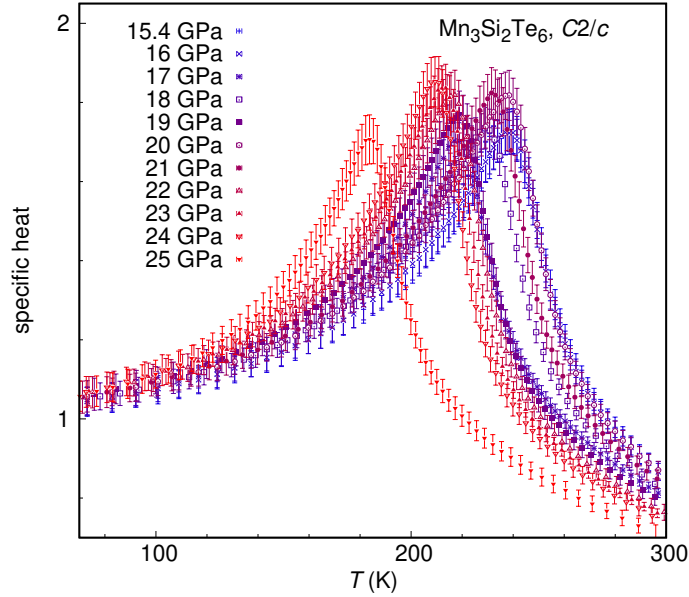

FIG. S5. Specific heat for the monoclinic  $C2/c$  structure of  $\text{Mn}_3\text{Si}_2\text{Te}_6$ . Pressures range from  $P = 15.4$  GPa to  $P = 25$  GPa.

We also present, in Figures S6 and S7, the magnetization curves as function of temperature for all pressure values we considered. The magnetization value  $1/3$  corresponds to the ferrimagnetic state where Mn trimers are in an up-down-up state and all trimers in the lattice are ferromagnetically ordered. In the monoclinic phase, some frustration in the Hamiltonian leads to a small modulation of the ferrimagnetic state so that the total magnetization for example for 15.4, 16 and 17 GPa does not reach the full  $1/3$ .

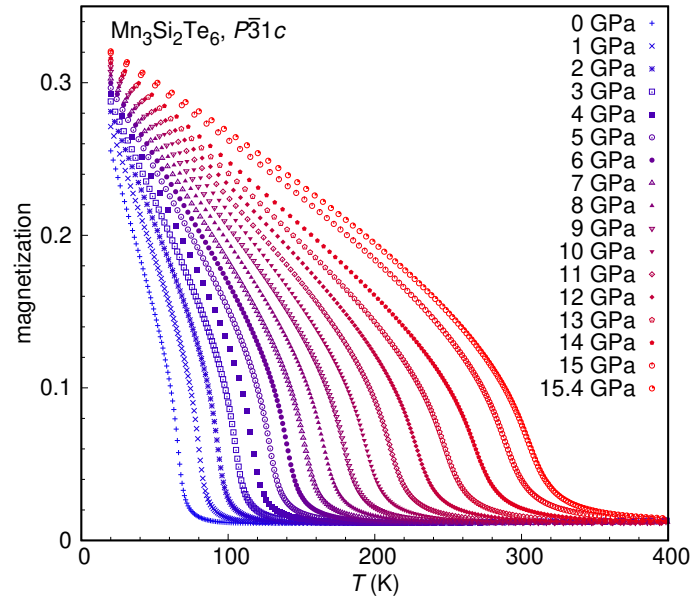

FIG. S6. Absolute value of the unit cell magnetization for the  $P\bar{3}1c$  structure of  $\text{Mn}_3\text{Si}_2\text{Te}_6$ . Pressures range from  $P = 0$  to  $P = 15.4$  GPa. The value  $1/3$  corresponds to the ferrimagnetic state.

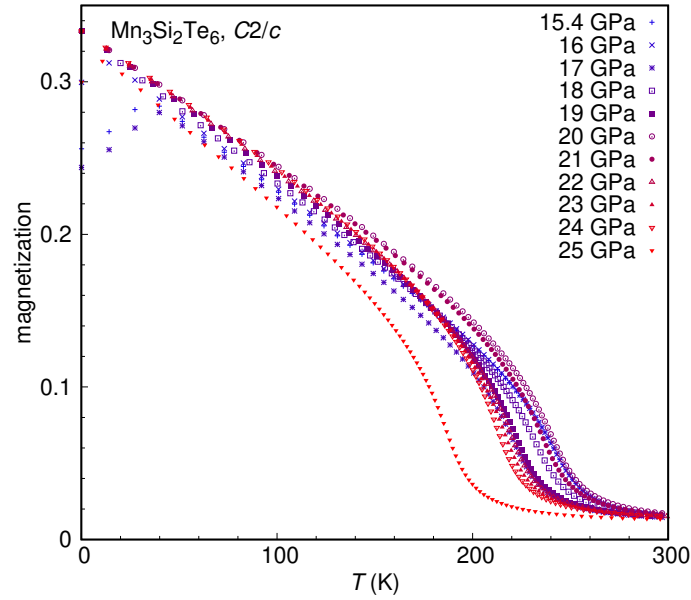

FIG. S7. Absolute value of the unit cell magnetization for the  $C2/c$  structure of  $\text{Mn}_3\text{Si}_2\text{Te}_6$ . Pressures range from  $P = 15.4$  GPa to  $P = 25$  GPa. The value  $1/3$  corresponds to the ferrimagnetic state.

- 
- [1] R. A. Susilo, C. I. Kwon, Y. Lee, N. P. Salke, C. De, J. Seo, B. Kang, R. J. Hemley, P. Dalladay-Simpson, Z. Wang, D. Y. Kim, K. Kim, S.-W. Cheong, H. W. Yeom, K. H. Kim, and J. S. Kim, High-temperature concomitant metal-insulator and spin-reorientation transitions in a compressed nodal-line ferrimagnet  $\text{Mn}_3\text{Si}_2\text{Te}_6$ , [Nat. Commun. \*\*15\*\*, 3998 \(2024\)](#).
